# Supplementary material for: Vulnerable GPU Memory Management: Towards Recovering Raw Data from GPU
Source: arXiv:1605.06610 source file (2016-05-21)
Supplement: Supplementary file 1 [file appendix.tex]

\appendix
